# Supplementary material for: Learning to Prevent Leakage: Privacy-Preserving Inference in the Mobile Cloud
Source: arXiv:1912.08421 source file (2021-06-15)
Supplement: Supplementary file 1 [file appendix.tex]

%\subsection{Compression techniques}
%\begin{itemize}
%	\item $F_{1}$(SVD)\cite{lane2016deepx}: This method inserts a fully-connected (FC) layer between two adjacent FC layers using singular value decomposition (SVD) based weight matrix factorization. We set the number of neurons in the inserted layers as $m/12$ where $m$ is the number of neurons of the first FC layer.
%	\item $F_{2}$~(KSVD)\cite{bhattacharya2016sparsification}: The method inserts a fully-connected (FC) layer between two adjacent FC layers using sparse coding. We set the number of neurons in the inserted layers as $m/6$ where $m$ is the number of neurons of the first FC layer.
%	\item $C_{1}$~(MobileNet)\cite{howard2017mobilenets}: This method 
%\end{itemize}
%
%
%
%$C_{1}$~(MobileNet)\cite{howard2017mobilenets}
%$C_{2}$~(MobileNetV2)\cite{sandler2018mobilenetv2}
%$C_{3}$~(SqueezeNet)\cite{iandola2016squeezenet}
%$W_{1}$~(Pruning)\cite{han2015deep}
%$W_{2}$~(Filter Pruning)\cite{li2016pruning}

%\section{Adversarial Retraining}
%We apply retraining strategies(i.e., reactive decoder and proactive decoder) to calculate the reward after getting actions. In this part, we present one training example of proactive decoder to show that proactive retraining indeed can get `private' features. Fig.~\ref{fig:mini}-(a)(c)(e) demonstrate an example proactive training process on CIFAR-10, VGG-16. As we observe, the overall model accuracy is high and stable throughout the training process, while the decoder and encoder pit against each other on the privacy loss with the encoder at an advantage. Fig.~\ref{fig:mini}-(b)(d)(f) shows the proactive training on CIFAR-100, VGG-16. Similarly, the decoder accuracy decays at the $20th$ epoch as the encoder gets stronger. The overall model accuracy remains stable.
%\begin{figure}[h]
%	\centering
%	\begin{minipage}[t]{0.48\linewidth}
%		\centering			\includegraphics[width=1\linewidth]{figures/experiment/cloud1.png}
%	\end{minipage}%
%	\begin{minipage}[t]{0.48\linewidth}
%		\centering			\includegraphics[width=1\linewidth]{figures/experiment/100c.png}
%	\end{minipage}
%	\centering
%	\begin{minipage}[t]{0.48\linewidth}
%		\centering			\includegraphics[width=1\linewidth]{figures/experiment/decoder1.png}
%	\end{minipage}%
%	\begin{minipage}[t]{0.48\linewidth}
%		\centering			\includegraphics[width=1\linewidth]{figures/experiment/100d.png}
%	\end{minipage}%
%	\label{fig:m2}
%	\centering
%	\begin{minipage}[t]{0.48\linewidth}
%		\centering			\includegraphics[width=1\linewidth]{figures/experiment/encoder_acc1.png}
%	\end{minipage}%
%	\begin{minipage}[t]{0.48\linewidth}
%		\centering			\includegraphics[width=1\linewidth]{figures/experiment/100e.png}
%	\end{minipage}%
%	\caption{
%		We partition VGG-16 at Layer 13 (left) and at Layer 33 (right), and then use filter pruning to compress the encoder. On the left side, the proactive decoder tries to maximize the SSIM to reconstruct the inputs. On the right side, the proactive decoder tries to minimize its classification error on the fine attributes to infer input properties.}
%	\label{fig:mini}
%\end{figure}
%% you can choose not to have a title for an appendix
%% if you want by leaving the argument blank
%{\color{red}\subsubsection{DQN}
%	Apart from policy gradient, we also implement	
%	\begin{figure}[h]
%		\centering
%		\begin{minipage}[t]{0.48\linewidth}
%			\centering	\includegraphics[width=1\linewidth]{figures/experiment/dqn_vgg11_reactive_para_cifar10.eps}
%		\end{minipage}
%		
%		\caption{DQN vs Policy gradient. Left: AlexNet todo; Right: VGG11 reactive parameter cifar10}
%		\label{fig:dqn}
%	\end{figure}
%	Policy gradient has better convergence performance. no time advantage.	
%}
%
%
%\section{Transfer learning example}
%\section{Decoder structure example}
%
%\section{Compression techniques details}
%TODO:
